# Supplementary material for: Acoustic Analogy of Quantum Baldin Sum Rule for Optimal Causal Scattering
Source: arXiv:2601.02630 ancillary file (2026-04-16)
Supplement: Supplementary file 1 [file SM_template.pdf]

# Supplementary Material

## Acoustic Analogy of Quantum Baldin Sum Rule for Optimal Causal Scattering

### Contents

|                                                                             |    |
|-----------------------------------------------------------------------------|----|
| S1. Theory of causality, multiple scattering and acoustic Baldin sum rule   | 1  |
| S1-1. Transmission coefficient derived from time reversal picture           | 1  |
| S1-2. Analytical validation for ideal point scatterers                      | 4  |
| S2. The calculation methods of the static bound                             | 7  |
| S2-1. Dispersion models for general and Fano resonators                     | 7  |
| S2-2. Closed-form models based on geometric parameters                      | 8  |
| S2-3. Numerical extract methods                                             | 9  |
| S3. Numerical simulation details                                            | 9  |
| S3-1. Underwater metamaterial I: the monopole Helmholtz resonator           | 10 |
| S3-2. Underwater metamaterial II: the dipole lead-core resonator            | 10 |
| S3-3. Parameters of airborne sound resonators (foam, Helmholtz, Fano types) | 11 |
| S3-4. Time-domain simulation (Helmholtz and Fano types)                     | 13 |
| S4. Impedance tube measurements                                             | 14 |
| S4-1. Sample fabrication                                                    | 14 |
| S4-2. Experimental setup: standard four microphone method                   | 15 |
| S4-3. Data post-processing: sum-rule-based Padé model fitting               | 15 |
| S4-4. Additional analysis of the measured data                              | 17 |
| References                                                                  | 18 |

### S1. Theory of causality, multiple scattering and acoustic Baldin sum rule

To establish the theory of causality, multiple scattering, and the acoustic analogy of quantum Baldin sum rule [1, 2], we first consider the homogenization problem (or effective medium theory) to facilitate our analysis. In real acoustic structures, there exists a uniquely corresponding homogenized density and modulus that yield identical responses, specifically in terms of the transmission and reflection coefficients [3]. This premise remains valid even in the high-frequency regime, extending beyond subwavelength considerations for one-dimensional scattering [4]. Consequently, we can derive an analytical expression for the transmission coefficient applicable to both normal and oblique incidence.

#### S1-1. Transmission coefficient derived from time reversal picture

We start by considering a 1D homogenized scatterer (characterized by  $\rho_{\text{eff}}$  and  $M_{\text{eff}}$ ), embedded in a background fluid with  $\rho_0$  and  $K_0$  (e.g., air or water). The background fluid is isotropic with density  $\rho_0$  and sound speed  $c_0$ . As plotted in Fig. (S1a), the total transmitted wave can be expressed

as the sum of all transmitted events:

$$T(\omega) = tt' \left( e^{ik_{\text{eff}}L} + r'^2 e^{3ik_{\text{eff}}L} + r'^4 e^{5ik_{\text{eff}}L} + \dots \right), \quad (\text{S1})$$

where the effective wavenumber  $k_{\text{eff}} = \omega \sqrt{\rho_{\text{eff}}/M_{\text{eff}}}$ , the interface reflection coefficient  $r' = (Z_0 - Z_{\text{eff}})/(Z_{\text{eff}} + Z_0)$  and the interface transmission coefficients are  $t = 2Z_{\text{eff}}/(Z_{\text{eff}} + Z_0)$  and  $t' = 2Z_0/(Z_{\text{eff}} + Z_0)$  (the primed coefficients denote transmission from the scatterer to the background fluid). The inverse Fourier transform of Eq. (S1) is given by

$$G(t) = \frac{1}{\sqrt{2\pi}} \int_{-\infty}^{\infty} T(\omega) e^{-i\omega t} d\omega. \quad (\text{S2})$$

By using the definition of the Dirac delta function, we obtain

$$G(t) = \frac{tt'}{\sqrt{2\pi}} \left[ \delta(t - \tau) + r'^2 \delta(t - 3\tau) + r'^4 \delta(t - 5\tau) + \dots \right], \quad (\text{S3})$$

where  $\tau = L/c_{\text{eff}} = L\sqrt{M_{\text{eff}}/\rho_{\text{eff}}}$ . The equally spaced centers of  $\delta$  functions represent transmission events at different times, while the dashed lines represent exponential energy loss due to impedance mismatch at the interfaces. Passivity requires that  $|r'|^2 < 1$  and  $|tt'| < 1$ .

If we reverse time [Fig. (S1b)], the physical picture is that the transmitted wave  $p_t$  at the present moment  $t_0$  is the superposition of the incident waves  $p_i$  at different times:  $p_t(t_0) = \int_0^{\infty} G(t) p_i(t_0 - t) d\tau$ . Causality dictates that the future cannot have any impact on the current moment, i.e.,  $G(t < 0) = 0$ . By carrying out the Fourier transform via  $p_{i/t}(\omega) = (1/\sqrt{2\pi}) \int_{-\infty}^{\infty} p_{i/t}(t) e^{i\omega t} dt$ , we obtain

$$T(\omega) = \frac{p_t(\omega)}{p_i(\omega)} = \frac{1}{\sqrt{2\pi}} \int_0^{\infty} G(t) e^{i\omega t} d\omega. \quad (\text{S4})$$

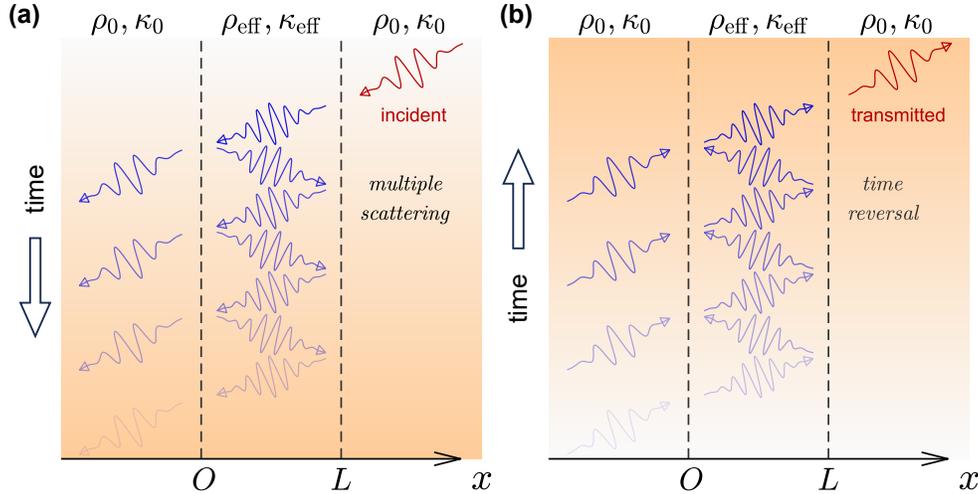

FIG. S1: The concept of scattering causality. (a) The multiple-scattering process of an incident pulse. (b) The time-reversed field yields a closed-form expression for the transmission coefficient. The figure illustrates the origin of the analytical nature of Eq. (S5), which arises from the time-delay response (causality). Note: The vertical axis represents time. This graph does not represent oblique incidence.

As evidenced by Eq. (S4), causality ensures that  $T(\omega)$  is *analytical* in the upper half-plane of the complex  $\omega$  (i.e., without any pole since  $G(t)$  is a real-valued time-domain causal kernel). By using the geometric series summation formula, Eq. (S1) can be converted to  $tt'e^{ik_{\text{eff}}L}/(1-r'^2e^{2ik_{\text{eff}}L})$ , which can be further simplified to Eq. (S5) (the same in the main text):

$$T(\omega) = \left[ \cos(k_{\text{eff}}L) - \frac{i}{2} \left( \frac{Z_{\text{eff}}}{Z_0} + \frac{Z_0}{Z_{\text{eff}}} \right) \sin(k_{\text{eff}}L) \right]^{-1}, \quad (\text{S5})$$

where  $Z_{\text{eff}} = \sqrt{\rho_{\text{eff}}M_{\text{eff}}}$ . In fact, the same expression for the transmission coefficient can be derived using the transfer matrix theory [5]. However, here we use the superposition and summation method of multiple scattering theory, which better reflects time delay and is closer to the actual physical picture.

According to  $\cos(k_{\text{eff}}L) \approx 1 - \frac{1}{2}(k_{\text{eff}}L)^2$  and  $\sin(k_{\text{eff}}L) \approx k_{\text{eff}}L$ , by taking the *subwavelength approximation* ( $k_{\text{eff}}L \ll 1$ ), Eq. (S5) can be approximated as

$$T(\omega) = \left[ 1 - \frac{1}{2}(k_{\text{eff}}L)^2 - \frac{i}{2} \left( \frac{Z_{\text{eff}}}{Z_0} + \frac{Z_0}{Z_{\text{eff}}} \right) (k_{\text{eff}}L) \right]^{-1} \quad (\text{S6})$$

and

$$T(\omega) \approx 1 + \frac{i}{2} \left( \frac{Z_{\text{eff}}}{Z_0} + \frac{Z_0}{Z_{\text{eff}}} \right) (k_{\text{eff}}L) + \left[ \frac{1}{2} - \frac{1}{4} \left( \frac{Z_{\text{eff}}}{Z_0} + \frac{Z_0}{Z_{\text{eff}}} \right)^2 \right] (k_{\text{eff}}L)^2. \quad (\text{S7})$$

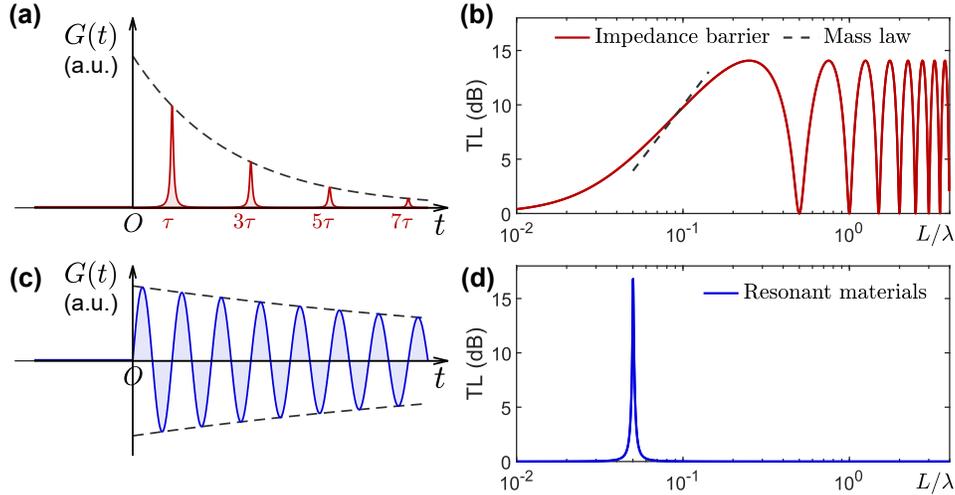

FIG. S2: Response functions  $G(t)$  [see Eq. (S2)] and the corresponding transmission loss (TL) (numerical validation). (a–b) Results for an impedance barrier with  $\frac{\rho_{\text{eff}}}{\rho_0} = 10$  and  $\frac{K_0}{M_{\text{eff}}} = 10$ . The mass law for the impedance barrier is presented with dashed line:  $\text{TL} \approx 20 \log_{10} \left( \frac{\omega \rho_{\text{eff}} L}{2Z_0} \right)$ , which is only approximately valid for limited band. (c–d) Results for a resonant scatterer with  $\frac{K_0}{M_{\text{eff}}} = 1$ , and  $\frac{\rho_{\text{eff}}}{\rho_0} = 1 + \frac{0.5 \times \omega_d^2}{\omega_d^2 - \omega^2 - i\beta\omega}$ , where  $\omega_d = 0.05 \times \frac{2\pi L}{c_0}$  and  $\beta = 0.005 \times \frac{L}{c_0}$ .

Here, we set that

$$\Gamma = \frac{\pi L}{2c_0} \left( \frac{K_0}{M_{\text{eff}}(0)} + \frac{\rho_{\text{eff}}(0)}{\rho_0} \right), \quad (\text{S8})$$

where  $\Gamma = \Gamma_m + \Gamma_d = (\pi L/2c_0)K_0/M_{\text{eff}}(0) + (\pi L/2c_0)\rho_{\text{eff}}(0)/\rho_0$ , defined at the static limit ( $\omega \rightarrow 0$ ). Eq. (S5) can be expanded as a second-order Taylor series

$$T(\omega) = 1 + i\omega \frac{\Gamma_m + \Gamma_d}{\pi} - \omega^2 \frac{\Gamma_m^2 + \Gamma_d^2}{\pi^2} + i\mathcal{O}(\omega^3), \quad (\text{S9})$$

where the first-order coefficient is locked as  $\Gamma_m + \Gamma_d (= \Gamma)$  (sum rule's bound). The second-order coefficient is associated with the low-frequency asymptotic behavior  $\sigma_{\text{ext}}(\omega) = \omega^2 [2(\Gamma_m^2 + \Gamma_d^2)/\pi^2] + \mathcal{O}(\omega^4)$ .

According to the main text, Kramer-Kronig relations are

$$\text{Re}[T(\omega) - 1] = \frac{2}{\pi} \mathcal{P} \int_0^\infty \frac{\omega' \text{Im}[T(\omega') - 1]}{\omega'^2 - \omega^2} d\omega' \quad (\text{S10})$$

and

$$\text{Im}[T(\omega) - 1] = \frac{-2\omega}{\pi} \mathcal{P} \int_0^\infty \frac{\text{Re}[T(\omega') - 1]}{\omega'^2 - \omega^2} d\omega' \quad (\text{S11})$$

As we mentioned in main text,  $\lim_{\omega \rightarrow 0} T(\omega) = 1$  for arbitrary scatterers with finite thickness and material properties, Eq. (S10) yields  $\int_0^\infty \text{Im}[T(\omega) - 1] d\omega/\omega = 0$  (this is relatively trivial without the information of the bound). However, by inserting 1D optical theorem  $\sigma_{\text{ext}}(\omega) = 2 \text{Re}[1 - T(\omega)]$  into Eq. (S11) and taking  $\omega \rightarrow 0$ , we derive acoustic Baldin sum rule as given

$$\int_0^\infty \sigma_{\text{ext}}(\omega) \frac{d\omega}{\omega^2} = \Gamma. \quad (\text{S12})$$

We insert Eq. (S5) into Eq. (S12), and the numerical integration yields a result that is 99.9% of  $\Gamma$ , as computed using MATLAB.

Here, we selected two representative cases: an impedance barrier and a locally resonant scatterer, whose dispersion parameters (which determine the value of  $\Gamma$ ) are described in the caption of Fig. (S2). This figure also illustrates the limitations of the mass law, particularly when the density of the barrier wall is only one order of magnitude greater than that of the background fluid, indicating a weak high-impedance assumption. Notably, if the assumptions hold that  $Z_{\text{eff}} \gg Z_0$  and  $\omega \rho_{\text{eff}} L \gg Z_0$  (where  $\rho_{\text{eff}}$  is a real-valued constant), the transmission loss defined as  $\text{TL} = -10 \log_{10} |T(\omega)|^2$  can be approximated by the expression  $20 \log_{10} (\omega \rho_{\text{eff}} L / 2Z_0)$ , adhering to the mass law. However, the linear region of the mass law exists only within a very narrow frequency band, and the slope deviates somewhat from the actual ground truth, as indicated by the red curve.

## S1-2. Analytical validation for ideal point scatterers

Instead of employing the physical Kramer-Kronig relations, we can utilize direct mathematical integral identities—provable through the residue theorem [6]—to verify the acoustic Baldin sum

rule for two representative types of ideal point scatterers under the subwavelength approximation:

$$\text{An impedance barrier: } \xi(\omega) = \xi_0, \quad (\text{S13a})$$

$$\text{A single-mode resonator: } \xi(\omega) = \frac{\xi_0 \omega_0^2}{\omega_0^2 - \omega^2 - i\beta\omega}, \quad (\text{S13b})$$

where  $\xi_0$  is a nondispersive constant and  $\beta$  denotes the dissipation factor of the resonance. Specifically, analogous to dispersion models for dielectric constants, the transmission spectrum of an impedance barrier resembles the Debye relaxation model, while that of a single-mode resonator corresponds to the Lorentz model. By taking the *subwavelength approximation* ( $k_{\text{eff}}L \ll 1$  for a point scatterer). By combining Eq. (S13), Eq. (S6) and 1D optical theorem, for the two cases [Eq. (S13a) and Eq. (S13b)], we will prove that Eq. (S12) yields  $\int_0^\infty \sigma_{\text{ext}}(\omega) \frac{d\omega}{\omega^2} \equiv \frac{\pi L}{2c_0} \xi(0)$ , where  $\xi(\omega) = \frac{\rho_{\text{eff}}(\omega)}{\rho_0} + \frac{K_0}{M_{\text{eff}}(\omega)}$  (acoustic analogy of quantum sum rule, with the derivation case by case below).

1. For the impedance barrier characterized by  $\xi(\omega) = \xi_0$  (a non-dispersive constant), we combine the definitions:  $T(\omega) \approx \left[1 - i \frac{\omega L}{2c_0} \xi(\omega)\right]^{-1}$  and  $\sigma_{\text{ext}}(\omega) = 2 \text{Re}[1 - T(\omega)]$  to derive  $\sigma_{\text{ext}} = 2 \text{Re} \left[1 - \left(1 - i \frac{\omega L}{2c_0} \xi_0\right)^{-1}\right] = \frac{2\tilde{\omega}^2}{1 + \tilde{\omega}^2}$ , where  $\tilde{\omega} = \frac{\omega L}{2c_0} \xi_0$ , and  $\xi_0 = \xi(0)$ . This allows us to simplify the integral as follows:

$$\int_0^\infty \sigma_{\text{ext}} \frac{d\omega}{\omega^2} = \frac{L\xi_0}{c_0} \int_0^\infty \frac{1}{1 + \tilde{\omega}^2} d\tilde{\omega} = \frac{\pi L\xi_0}{2c_0}. \quad (\text{S14})$$

Here, we utilize the identity  $\int_0^\infty \frac{1}{1+x^2} dx = \frac{\pi}{2}$ . This is a standard integral whose antiderivative is known:  $\int \frac{1}{1+x^2} dx = \arctan(x) + C$ . Using the Fundamental Theorem of Calculus, we compute the definite integral:  $\int_0^\infty \frac{1}{1+x^2} dx = \lim_{b \rightarrow \infty} \int_0^b \frac{1}{1+x^2} dx = \lim_{b \rightarrow \infty} [\arctan(x)]_0^b$ . Since  $\arctan(0) = 0$  and  $\lim_{x \rightarrow \infty} \arctan(x) = \frac{\pi}{2}$ , we obtain  $\int_0^\infty \frac{1}{1+x^2} dx = \frac{\pi}{2}$ .

2. For a single-mode resonator with  $\xi(\omega) = \frac{\xi_0 \omega_0^2}{\omega_0^2 - \omega^2 - i\beta\omega}$ , we again combine the definitions:  $T(\omega) \approx \left[1 - i \frac{\omega L}{2c_0} \xi(\omega)\right]^{-1}$  and  $\sigma_{\text{ext}}(\omega) = 2 \text{Re}[1 - T(\omega)]$  to obtain

$$\sigma_{\text{ext}} = 2 \text{Re} \left[1 - \left(1 - i \frac{\omega L}{2c_0} \frac{\xi_0 \omega_0^2}{\omega_0^2 - \omega^2 - i\beta\omega}\right)^{-1}\right], \quad (\text{S15})$$

which can be simplified to  $\frac{2\omega^2 \alpha (\beta + \alpha)}{(\omega_0^2 - \omega^2)^2 + \omega^2 (\beta + \alpha)^2}$ , where  $\alpha = \frac{\xi_0 L \omega_0^2}{2c_0}$ . Continuing, we compute

$$\int_0^\infty \sigma_{\text{ext}} \frac{d\omega}{\omega^2} = \int_0^\infty \frac{2\alpha(\beta + \alpha)}{(\omega^2 - \omega_0^2)^2 + \omega^2(\beta + \alpha)^2} d\omega = \frac{\pi L \xi_0}{2c_0}. \quad (\text{S16})$$

This calculation employs the identity  $\int_0^\infty \frac{\mu x_0^2}{(x^2 - x_0^2)^2 + \mu^2 x^2} dx = \frac{\pi}{2}$ . Since the integrand is an even

function, we extend the range to  $(-\infty, \infty)$  and consider the complex function  $f(z)$ :

$$I = \frac{1}{2} \oint_C f(z) dz, \quad \text{where } f(z) = \frac{\mu x_0^2}{(z^2 - x_0^2)^2 + \mu^2 z^2}$$

We close the contour in the upper half-plane (UHP). The poles occur where  $(z^2 - x_0^2)^2 + \mu^2 z^2 = 0$ , which factors into  $(z^2 - i\mu z - x_0^2)(z^2 + i\mu z - x_0^2) = 0$ . Letting  $\Omega = \sqrt{4x_0^2 - \mu^2}$ , the two poles lying in the UHP are  $z_1 = \frac{\Omega + i\mu}{2}$  and  $z_2 = \frac{-\Omega + i\mu}{2}$ . Using the formula  $\text{Res}(f, z_k) = \lim_{z \rightarrow z_k} (z - z_k)f(z)$ , we find the residues to be  $\text{Res}(f, z_1) = \frac{x_0^2}{i\Omega(\Omega + i\mu)}$  and  $\text{Res}(f, z_2) = \frac{x_0^2}{i\Omega(\Omega - i\mu)}$ . Summing these residues:

$$\sum \text{Res} = \frac{x_0^2}{i\Omega} \left( \frac{1}{\Omega + i\mu} + \frac{1}{\Omega - i\mu} \right) = \frac{x_0^2}{i\Omega} \frac{2\Omega}{\Omega^2 + \mu^2}.$$

Substituting  $\Omega^2 + \mu^2 = 4x_0^2$ , the sum simplifies to:  $\sum \text{Res} = \frac{2x_0^2}{i(4x_0^2)} = \frac{1}{2i}$ . Finally, applying the Residue Theorem  $\int_{-\infty}^{\infty} f(x)dx = 2\pi i \sum \text{Res}$ :  $I = \frac{1}{2} (2\pi i \cdot \frac{1}{2i}) = \frac{\pi}{2}$ .

These two examples highlight the additional degrees of freedom in scattering dynamics. The sum rule provides theoretical insights on why metamaterials enable *deep subwavelength* wave manipulation. The modal design of metamaterials is essentially to concentrate higher frequency modes (characterized by  $\sigma_{\text{ext}}$ ) into low frequencies, but at the expense of bandwidth.

Finally, we look at an example without subwavelength approximation (non-ideal point scatterer):  $\rho_{\text{eff}} = \bar{\rho}$  and  $M_{\text{eff}} = \bar{K}$  (constants without frequency dependency). For simplicity, we assume this is transparent barrier without reflection:  $\sqrt{\rho_{\text{eff}} M_{\text{eff}}} = \sqrt{\bar{\rho} \bar{K}} = Z_0$  (impedance matched to the background fluid). Moreover,  $c_{\text{eff}} = \bar{c} = \sqrt{\bar{M}/\bar{\rho}}$  and  $k_{\text{eff}} = \bar{k} = \omega/\bar{c}$  (where  $\bar{c} \neq c_0$ ). According to Eq. (S5), the resulting transmission will be a phase-delayed complex-value:

$$T(\omega) = \exp(i\bar{k}L), \quad (\text{S17})$$

whose absolute value will be unity. By inserting this formula, into the Eq. (S12), the remaining task is to check  $\int_0^{\infty} \frac{2\text{Re}[1 - \exp(i\bar{k}L)]}{\omega^2} d\omega = \pi \frac{L}{\bar{c}}$ . If we set  $\bar{k}L$  as  $x$ , the integration can be written as  $\frac{L}{\bar{c}} \int_0^{\infty} \frac{2\text{Re}[1 - \exp(ix)]}{x^2} dx = \frac{L}{2\bar{c}} \int_{-\infty}^{\infty} \frac{2\text{Re}[1 - \exp(ix)]}{x^2} dx$  (because its real part is an even function). By using the identity  $I = \int_{-\infty}^{\infty} \frac{2\text{Re}(1 - e^{ix})}{x^2} = 2\pi$ , it is matched with the  $\Gamma = \frac{\pi L}{2c_0} \left( \frac{K_0}{M_{\text{eff}}(0)} + \frac{\rho_{\text{eff}}(0)}{\rho_0} \right) = \frac{\pi L}{2c_0} 2\sqrt{\frac{K_0}{M_{\text{eff}}(0)} \frac{\rho_{\text{eff}}(0)}{\rho_0}} = \pi \frac{L}{\bar{c}}$ . This final example demonstrates that the bound of the sum rule is essentially a cumulative phase.

Identity derivation: to evaluate the integral  $I = \int_{-\infty}^{\infty} \frac{2\text{Re}(1 - e^{ix})}{x^2} dx$ , we first simplify the integrand using Euler's formula  $e^{ix} = \cos x + i \sin x$ . The term  $1 - e^{ix}$  becomes  $1 - \cos x - i \sin x$ , so its real part is  $1 - \cos x$ . Using the half-angle identity  $1 - \cos x = 2 \sin^2(x/2)$ , the integral transforms into  $I = \int_{-\infty}^{\infty} \frac{2(2 \sin^2(x/2))}{x^2} dx = \int_{-\infty}^{\infty} \left( \frac{\sin(x/2)}{x/2} \right)^2 dx$ . By substituting  $u = x/2$ , where  $dx = 2 du$ , the integral becomes  $I = 2 \int_{-\infty}^{\infty} \frac{\sin^2 u}{u^2} du$ . Integrating by parts with  $f = \sin^2 u$ ,  $g' = 1/u^2$ , we

get  $f' = 2 \sin u \cos u = \sin(2u)$  and  $g = -1/u$ . The boundary term  $-\left[\frac{\sin^2 u}{u}\right]_{-\infty}^{\infty}$  vanishes, leaving  $I = 2 \int_{-\infty}^{\infty} \frac{\sin(2u)}{u} du$ . Finally, letting  $v = 2u$ , we arrive at  $I = 2 \int_{-\infty}^{\infty} \frac{\sin v}{v} dv$ . Using the Dirichlet integral result [6]  $\int_{-\infty}^{\infty} \frac{\sin v}{v} dv = \pi$ , we conclude that  $I = 2\pi$ .

## S2. The calculation methods of the static bound

To correctly evaluate the static bound  $\Gamma$  in sum rule, we introduce both general theoretical and numerical methods in this section.

### S2-1. Dispersion models for general and Fano resonators

The effective properties generally follow Lorentz model [3]:

$$\frac{K_0}{M_{\text{eff}}(\omega)} = \frac{2c_0}{L} \sum_{k=1}^M \frac{\alpha_{m,k}}{\omega_{m,k}^2 - \omega^2 - i\beta_{m,k}\omega}, \quad (\text{S18a})$$

$$\frac{\rho_{\text{eff}}(\omega)}{\rho_0} = \frac{2c_0}{L} \sum_{j=1}^N \frac{\alpha_{d,j}}{\omega_{d,j}^2 - \omega^2 - i\beta_{d,j}\omega}, \quad (\text{S18b})$$

where  $M, N$  denote the numbers of monopole and dipole oscillators, respectively. By inserting Eq. (S18) into Eq. (S6), we can derive a similar form, satisfying analyticity condition  $T(\omega) = T^*(-\omega)$ , like general Padé model:

$$2[1 - T(\omega)] = \frac{a_1(-i\omega) + a_2(-i\omega)^2 + \dots + a_m(-i\omega)^m}{1 + b_1(-i\omega) + b_2(-i\omega)^2 + \dots + b_n(-i\omega)^n}. \quad (\text{S19})$$

For the Fano resonator, the piston motion of narrowed channel contribute to a piston-like radiation mode [ $\rho_{\text{eff}}/\rho_0 \approx 1/\varphi = (2c_0/L)\sqrt{b}$ ], while the resonant monopole yields  $K_0/K_{\text{eff}}(\omega) = K_0/M_{\text{eff}}(\omega) = (2c_0/L)\alpha/(\omega_m^2 - \omega^2)$ . Therefore, an analytical asymptotic form

$$T(\omega) = \left[1 - i\omega \left(\sqrt{b} + \frac{\alpha}{\omega_m^2 - \omega^2 - i\beta\omega}\right)\right]^{-1}, \quad (\text{S20})$$

which coincide the spectral line-shape of the Fano transmission ( $\beta \rightarrow 0$ ), reported in Ref. [7]. The Fano scattering can be alternatively modeled as Padé model of order  $[3 \times 3]$ :

$$2[1 - T(\omega)] = \frac{a_1(-i\omega) + a_2(-i\omega)^2 + a_3(-i\omega)^3}{1 + b_1(-i\omega) + b_2(-i\omega)^2 + b_3(-i\omega)^3}, \quad (\text{S21})$$

where  $a_1 = 2(\sqrt{b} + \alpha/\omega_m^2)$ ,  $a_2 = 2\sqrt{b}\beta/\omega_m^2$ ,  $a_3 = 2\sqrt{b}/\omega_m^2$ ,  $b_1 = \sqrt{b} + (\alpha + \beta)/\omega_m^2$ ,  $b_2 = (\sqrt{b}\beta + 1)/\omega_m^2$ ,  $b_3 = \sqrt{b}/\omega_m^2$ . The conventional resonances of foam liner and Helmholtz resonator are featured by symmetrical lineshape of  $T(\omega)$  ( $\sqrt{b} = 0$ ) if the horizontal axis is  $\log(\omega)$  [see Fig. (S9)].

## S2-2. Closed-form models based on geometric parameters

We consider a three-dimensional periodic composite system characterized by a unit cell containing three distinct, isotropic, and linear elastic phases [Fig. (S3)]: a epoxy matrix ( $\Omega_1$ ), a rubber coating ( $\Omega_2$ ), and a lead core ( $\Omega_3$ ). Within each phase  $m$  ( $m = 1, 2, 3$ ), the material properties—density  $\rho_m$  and Lamé parameters  $\lambda_m, \mu_m$ —are constant. The displacement field  $\mathbf{u}(\mathbf{r})$  within each homogeneous region  $\Omega_m$  (assuming a time-harmonic dependence  $e^{-i\omega t}$ ) is governed by elastic wave equation [8]:

$$(\lambda_m + \mu_m)\nabla(\nabla \cdot \mathbf{u}) + \mu_m \nabla^2 \mathbf{u} + \rho_m \omega^2 \mathbf{u} = 0, \quad \text{for } \mathbf{r} \in \Omega_m, \quad (\text{S22})$$

where  $\nabla^2$  is the vector Laplacian operator. The mechanical parameters for FEM simulation are listed in Table (S2). According to Ref. [9], the static effective density of the composite is defined by the volume average:

$$\rho_{\text{eff}} = f_1 \rho_1 + f_2 \rho_2 + f_3 \rho_3, \quad (\text{S23})$$

where  $f_1, f_2$ , and  $f_3$  denote the volume fractions of the matrix, rubber coating, and lead core, respectively. If the matrix is a fluid ( $\Omega_1$ ), Eq. (S23) should be corrected by using Berryman equations [10] (not volume average). For dipole underwater mechanical metamaterial, static  $M_{\text{eff}}$  is not the same as the P-wave modulus  $K_{\text{eff}}(0)$ , due to the shear component  $\mu_{\text{eff}}$ , which is determined by

$$M_{\text{eff}} = K_{\text{eff}} + 4\mu_{\text{eff}}/3, \quad (\text{S24})$$

where the effective bulk modulus  $K_{\text{eff}}$  is calculated using a nested scheme. First, the bulk modulus of the coated inclusion is given by  $K_p = K_2 + \frac{\phi(K_3 - K_2)}{1 + 3(1 - \phi)[(K_3 - K_2)/(3K_2 + 4\mu_2)]}$ , where  $\phi = \frac{f_3}{f_2 + f_3}$ . Subsequently, the overall effective bulk modulus is  $K_{\text{eff}} = K_1 + \frac{(1 - f_1)(K_p - K_1)}{1 + 3f_1(K_p - K_1)/(3K_1 + 4\mu_1)}$ . Similarly, the effective shear modulus  $\mu_{\text{eff}} = \mu_1 + \frac{5(1 - f_1)\mu_1(\mu_p - \mu_1)}{5\mu_1 + 6f_1(\mu_p - \mu_1)[(K_1 + 2\mu_1)/(3K_1 + 4\mu_1)]}$ , where the shear modulus of the coated inclusion is defined as  $\mu_p = \mu_2 + \frac{5f_3(\mu_3 - \mu_2)\mu_2}{5(f_3 + f_2)\mu_2 + 6f_2(\mu_3 - \mu_2)[(K_2 + 2\mu_2)/(3K_2 + 4\mu_2)]}$ .

For fluid-based resonators, according to the analytical model of perforated pores [5, 11] and Wood's formula [3, 12], the static effective parameters are given by

$$\frac{\rho_{\text{eff}}(0)}{\rho_0} = \frac{L + \Delta L}{\varphi L}, \quad (\text{S25a})$$

$$\frac{K_0}{K_{\text{eff}}(0)} = \frac{V_{\text{eff}}}{S_0 L}, \quad (\text{S25b})$$

where the sample thickness is  $L$ ,  $S_0$  is the main duct cross-sectional area, the end correction  $\Delta L = (16/(3\pi))\sqrt{\varphi S_0/\pi}F(\varphi)$ . Here, the definition of Fok function  $F(\varphi)$  is [5]

$$F(\phi) = 1 - 1.41\phi^{\frac{1}{2}} + 0.34\phi^{\frac{3}{2}} + 0.07\phi^{\frac{5}{2}} - 0.02\phi^3 + 0.03\phi^{\frac{7}{2}}, \quad (\text{S26})$$

where  $\varphi S_0$  is the cross-sectional area of the narrowed channel with perforation ratio  $\varphi$  (or ventilation rate). Here,  $V_{\text{eff}}$  denotes the total effective volume of the fluid domain, which should be evaluated differently in pure fluid and porous domains (for foam liner), i.e.,  $V_{\text{eff}} = V_{\text{fluid}}^0 + V_{\text{poro}}$ . The actual fluid-occupied volume of main duct is simply  $V_{\text{fluid}}^0$ . In the porous domain, due to the static interaction between microstructures and viscous boundary layers, the fluid motion inside the porous material is isothermal, according to Ref. [12]. Accordingly,  $V_{\text{poro}} = \gamma_{\text{fluid}} V_{\text{liner}}^0 \phi$ , where  $V_{\text{liner}}^0$  is the total volume of the liner without porous materials,  $\phi$  is the porosity excluding the skeleton volume

of the porous structure, and  $\gamma_{\text{fluid}}$  is the adiabatic index of the fluid (for air,  $\gamma_{\text{fluid}} = 1.4$ ).

### S2-3. Numerical extract methods

The simulated reflection, and transmission coefficients [ $R(\omega)$  and  $T(\omega)$ ] were defined at the front and back surfaces of the sample, respectively. These coefficients facilitated the extraction of effective P-wave modulus and effective density spectra ( $\frac{K_0}{M_{\text{eff}}(\omega)}$  and  $\frac{\rho_{\text{eff}}(\omega)}{\rho_0}$ ), utilizing the formula outlined in Ref. [3] and Table (S1). It is crucial to distinguish these coefficients from the S-parameters (acpr. $S_{11}$  and acpr. $S_{21}$  extracted from the FEM simulation in the acpr model of pressure acoustics frequency domain), which are directly defined at the surfaces of the input and output ports. The relationships are expressed as  $R(\omega) = \text{acpr}.S_{11} \times e^{-2ik_0L_{\text{dist}}}$  (or  $S_{11}$ ) and  $T(\omega) = \text{acpr}.S_{21} \times e^{-2ik_0L_{\text{dist}}}$  (or  $S_{21}$ ) [ $L_{\text{dist}}$  is the distance between the sample surface to the input or output port].

### S3. Numerical simulation details

Simulation was carried out using the COMSOL Multiphysics commercial software, specifically employing the finite element method (FEM) facilitated through the 'Pressure Acoustics, Frequency Domain' module. The simulation setup included monitoring of incident and transmitted waves via two ports located at the boundaries of the model. In cases where the cavity of the liner were filled with a highly absorptive porous foam [11], the Johnson-Champoux-Allard (JCA) model was

| Name                | Expression                                                                       | Unit                  | Description                         |
|---------------------|----------------------------------------------------------------------------------|-----------------------|-------------------------------------|
| $S_{11}$            | $\text{acpr}.S_{11} \cdot e^{2ik_0L_{\text{dist}}}$                              | –                     | From port 1 to sample front surface |
| $S_{21}$            | $\text{acpr}.S_{21} \cdot e^{2ik_0L_{\text{dist}}}$                              | –                     | From port 2 to sample back surface  |
| $\rho_{\text{eff}}$ | $\frac{4i \cdot t_{12}}{\text{acpr}.\omega \cdot L \cdot (2 + t_{11} + t_{22})}$ | kg/m <sup>3</sup>     | Effective density formula           |
| $C_{\text{eff}}$    | $\frac{4i \cdot t_{21}}{\text{acpr}.\omega \cdot L \cdot (2 + t_{11} + t_{22})}$ | 1/Pa                  | Effective compressibility formula   |
| $K_{\text{eff}}$    | $1/C_{\text{eff}}$                                                               | Pa                    | Effective modulus formula           |
| $k_0$               | $\text{acpr}.\omega/c_0$                                                         | rad/m                 | Wavenumber for incident wave        |
| $A$                 | $\frac{(1 + S_{11})(1 - S_{11}) + S_{21}^2}{2S_{21}}$                            | –                     | A element from ABCD matrix          |
| $B$                 | $\frac{Z_0((1 + S_{11})(1 + S_{11}) - S_{11}^2)}{2S_{21}}$                       | kg/(m <sup>2</sup> s) | B element from ABCD matrix          |
| $C$                 | $\frac{(1 - S_{11})(1 - S_{11}) - S_{21}^2}{2S_{21}Z_0}$                         | m <sup>2</sup> s/kg   | C element from ABCD matrix          |
| $D$                 | $\frac{(1 - S_{11})(1 + S_{11}) + S_{21}^2}{2S_{21}}$                            | –                     | D element from ABCD matrix          |
| $t_{11}$            | $D$                                                                              | –                     | Notation conversion 1 (T-matrix)    |
| $t_{12}$            | $-B$                                                                             | kg/(m <sup>2</sup> s) | Notation conversion 2 (T-matrix)    |
| $t_{21}$            | $-C$                                                                             | m <sup>2</sup> s/kg   | Notation conversion 3 (T-matrix)    |
| $t_{22}$            | $A$                                                                              | –                     | Notation conversion 4 (T-matrix)    |

TABLE S1: The algorithm variables [3] for extracting the effective dynamic parameters  $\rho_{\text{eff}}$  and  $M_{\text{eff}}$  from the reflection ( $S_{11}$ ) and transmission ( $S_{21}$ ) data obtained in the simulation software, which can be converted to the ABCD matrix. acpr.S21 and acpr.S11 are the transmission and reflection coefficients defined at the ports. A phase correction factor  $e^{2ik_0L_{\text{dist}}}$  is applied to account for the (double) distance between the front (or back) surface of the sample and the incident (or output) port.

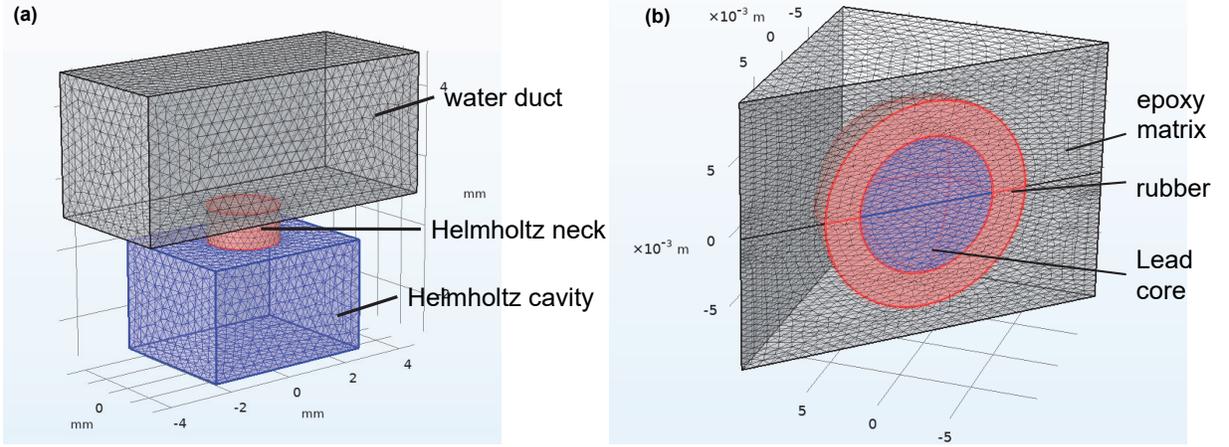

FIG. S3: The practical FEM mesh model used for simulating the underwater metamaterials with monopole and dipole resonator configurations. The dipole model is presented with a reduced half geometry for the view of the embedded layers.

TABLE S2: Material parameters for the three-phase locally resonant sonic material.

| Phase            | Symbol     | Density $\rho$ (kg/m <sup>3</sup> ) | 1st Lamé $\lambda$ (Pa) | Shear $\mu$ (Pa)      |
|------------------|------------|-------------------------------------|-------------------------|-----------------------|
| Matrix (Epoxy)   | $\Omega_1$ | $1.18 \times 10^3$                  | $4.43 \times 10^9$      | $1.59 \times 10^9$    |
| Coating (Rubber) | $\Omega_2$ | $1.30 \times 10^3$                  | $6.00 \times 10^5$      | $4.00 \times 10^4$    |
| Core (Lead)      | $\Omega_3$ | $19.3 \times 10^3$                  | $4.23 \times 10^{10}$   | $1.49 \times 10^{10}$ |

utilized, characterized by the following parameters (also adopted from Ref. [11]): porosity  $\varphi = 0.94$ , fluid resistance  $R_f = 32000[\text{Pa} \cdot \text{s}/\text{m}^2]$ , tortuosity factor  $\alpha_\infty = 1.06$ , viscous characteristic length  $L_v = 56[\mu\text{m}]$ , thermal characteristic length  $L_{\text{th}} = 110[\mu\text{m}]$ .

### S3-1. Underwater metamaterial I: the monopole Helmholtz resonator

In original ultrasonic metamaterial experiment [13], the basic unit is a Helmholtz resonator fabricated from aluminum wall (thick enough to form an ultrasound waveguide). The resonator consists of a rectangular cavity with dimensions of  $3.14 \text{ mm} \times 4 \text{ mm} \times 5 \text{ mm}$  and a cylindrical neck that is  $1 \text{ mm}$  in length and  $1 \text{ mm}$  in diameter. Both the cavity and neck are filled with water and connected on the same side to a square water duct with a cross-sectional area of  $4 \text{ mm} \times 4 \text{ mm}$ . The Helmholtz resonators are arranged in a periodic array with a spacing of  $9.2 \text{ mm}$ , forming a one-dimensional daisy-chained structure used to realize an acoustic metamaterial with negative effective modulus. Here, we only simulated one unit cell with its thickness the same as  $L = 9.2 \text{ mm}$ , with other parameters unchanged, as shown in Fig. (S3a).

### S3-2. Underwater metamaterial II: the dipole lead-core resonator

In Fig. (S3b), we consider a three-dimensional periodic composite system characterized by a cubic unit cell with lattice constant  $a$ . According to the parameters described in Ref. [14], the unit cell contains a spherical inclusion composed of three distinct, isotropic, and linear elastic phases: the matrix ( $\Omega_1$ , epoxy), the coating ( $\Omega_2$ , rubber), and the core ( $\Omega_3$ , metal). The geometric parameters

are determined by the filling ratio  $\phi = 0.48$ . The core diameter is defined as  $d_{\text{lead}} = 1$  cm, and the rubber coating thickness is  $d_{\text{rubber}} = 0.25$  cm. Consequently, the lattice constant  $a$  is derived to satisfy the filling ratio requirement:

$$a = \sqrt{\frac{\pi(d_{\text{lead}}/2 + d_{\text{rubber}})^2}{\phi}} = 1.9 \text{ cm.} \quad (\text{S27})$$

The simulation domain includes a tube length  $L_{\text{tube}} = 5a$ , surrounded by a water domain with sound speed  $c_0 = 1500$  m/s and density  $\rho_0 = 1000$  kg/m<sup>3</sup>. Within each phase  $m$  ( $m = 1, 2, 3$ ), the material properties—density  $\rho_m$  and Lamé parameters  $\lambda_m, \mu_m$ —are constant. The specific material parameters used in the numerical model are listed in Table (S2). The bulk modulus for each phase is calculated as  $K_m = \lambda_m + 2\mu_m/3$ . To validate the acoustic performance, we calculate the effective dynamic properties of the composite. The volume fractions for the metal core ( $f_3$ ), rubber coating ( $f_2$ ), and matrix ( $f_1$ ) are calculated geometrically based on the spherical radii relative to the unit cell volume  $a^3$ . The related results are listed in End Matter in the main text.

### S3-3. Parameters of airborne sound resonators (foam, Helmholtz, Fano types)

Our design is predicated on the sum rule principle without the application of sophisticated optimization techniques. To ensure simplicity, all designs are characterized by a two-dimensional axis-symmetrical geometry. This approach allows for the reconstruction of the three-dimensional structure through rotation around the central axis of the main duct, with a diameter of 3 cm ( $S_0 = \pi(1.5[\text{cm}])^2$ ). For all samples illustrated in [Fig. (S8a)], the thickness is uniformly set at  $L = 2.5$  cm.

As illustrated in Fig. (S4), the primary concept is the construction of an effective density that exceeds that of the background through the implementation of a narrowed channel. This phenomenon is analogous to a pure mass barrier, akin to piston motion within a perforated pore. Additionally, by utilizing the supplementary volume from the lateral structures of the main duct—such as liners or resonators mounted on the waveguide wall—we can enhance the volume of the scatterer, thus creating a local resonant state. The interplay between discrete states and the continuum background represents the fundamental components necessary for the construction of a Fano resonator.

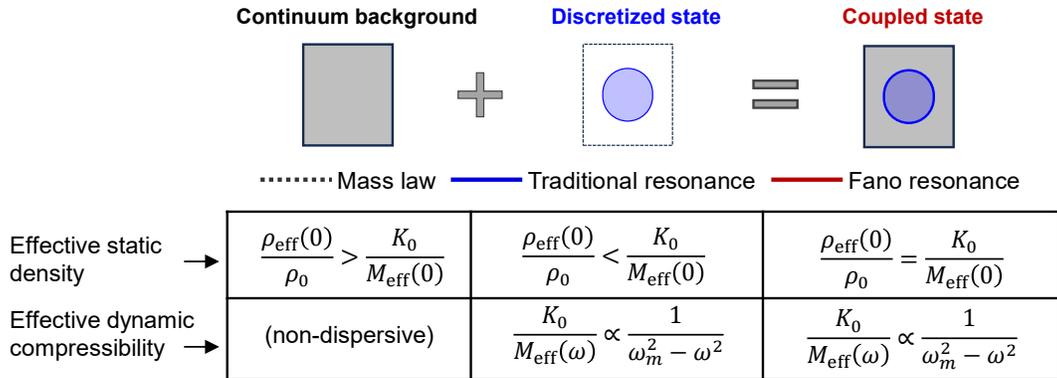

FIG. S4: The concept of Fano resonance, which can be interpreted as the interference between a continuum background (e.g., a dipole resonance with near-zero frequency and significant radiation loss) and a discrete state (e.g., a localized Helmholtz resonance).

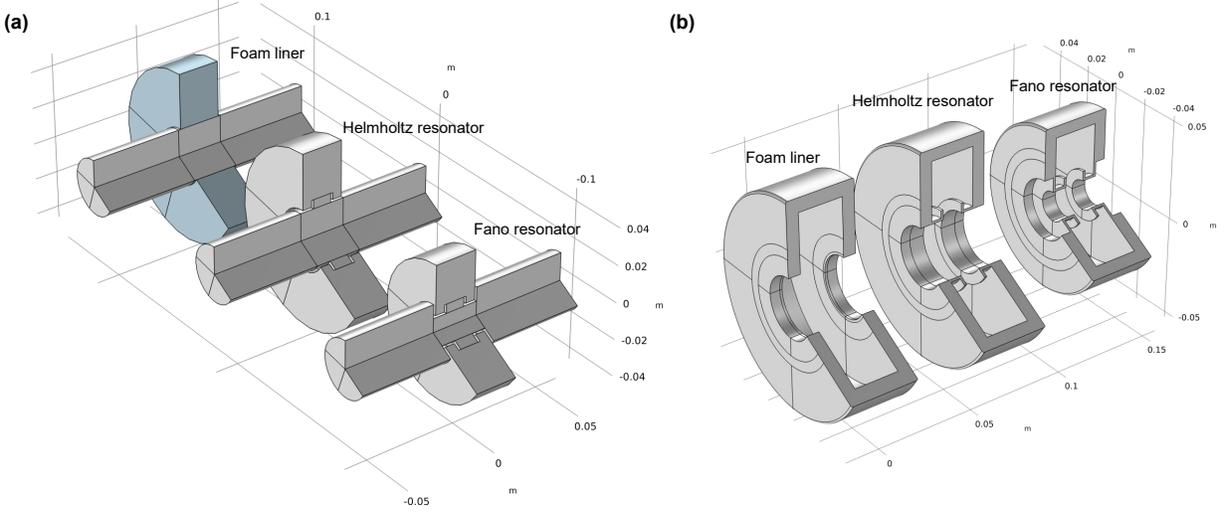

FIG. S5: The geometry models of the foam liner, Helmholtz resonator, and optimal Fano resonator. (a) The simulated air domain, including the porous foam region. (b) The 3D-printed resonator sample, with rigid walls made of solid resin.

Initially, the geometry of the foam liner is established without a specific preference. The foam liner is designed with a cavity height of 3.05 cm and a width of 2.26 cm, which is constrained to be less than the 3 cm thickness due to the presence of a 0.7 mm solid frame partition. The total volume of the liner cavity is calculated to be  $1.3 \times 10^{-4} \text{m}^3$ . When combined with the volume of the main duct, the total volume amounts to  $1.47 \times 10^{-4} \text{m}^3$ , which should be differentiated from  $V_{\text{eff}}$  as discussed in the main text. It is noted that the volume of the porous region must be multiplied by the adiabatic index of the fluid, where for air,  $\gamma_{\text{fluid}} = 1.4$ . Consequently, for an air-based structure,  $V_{\text{eff}} = 1.3 \times 10^{-4} \text{m}^3 \times 1.4 + 0.17 \times 10^{-4} \text{m}^3$ . As a result, we obtain  $\xi(0) = K_0/K_{\text{eff}}(0) + \rho_{\text{eff}}(0)/\rho_0 = 8.32 \times 1.4 + 1 = 12.65$ .

Next, the Helmholtz resonator is constructed with a cavity volume (including the neck volume) equal to the foam liner's volume of  $1.3 \times 10^{-4} \text{m}^3$ . Consequently, the total volume, comprising both the cavity and the main duct volume ( $S_0 \times L$ ), remains consistent at  $1.47 \times 10^{-4} \text{m}^3$ . The dimensions of the Helmholtz neck are chosen to be 5 mm in height and 10 mm in width, with the neck embedded within the cavity to minimize space wastage. The height of the Helmholtz cavity is calculated to be 2.66 cm, while the width remains at 2.26 cm, congruent with that of the foam liner. It is observed that  $K_0/K_{\text{eff}}(0) \approx \frac{1.47 \times 10^{-4} \text{m}^3}{S_0 L} = 8.32$ . For effective density, we find  $\rho_{\text{eff}}(0)/\rho_0 \approx 1$ . Hence,  $\xi(0) = K_0/K_{\text{eff}}(0) + \rho_{\text{eff}}(0)/\rho_0 = 9.32$ .

Lastly, the Fano resonator is constructed with a ventilation rate of  $\varphi = 0.25$ , leading to an effective density ratio of  $\rho_{\text{eff}}(0)/\rho_0 \approx 9.32/2 = 4.66$ . To maintain a consistent total  $\xi(0)$  between the Fano and Helmholtz resonators, it is requisite that  $K_0/K_{\text{eff}}(0) = 4.66$ . This condition facilitates optimal Fano interference, minimizing low-frequency scattering while maximizing sound insulation in higher frequency bands. The embedded neck dimensions of the Fano resonator are identical to those of the Helmholtz resonator; however, its cavity features a height of 2.66 cm (calculated inversely) and a width of 2.26 cm (fixed) to satisfy the condition of  $K_0/K_{\text{eff}}(0) = 4.66$ .

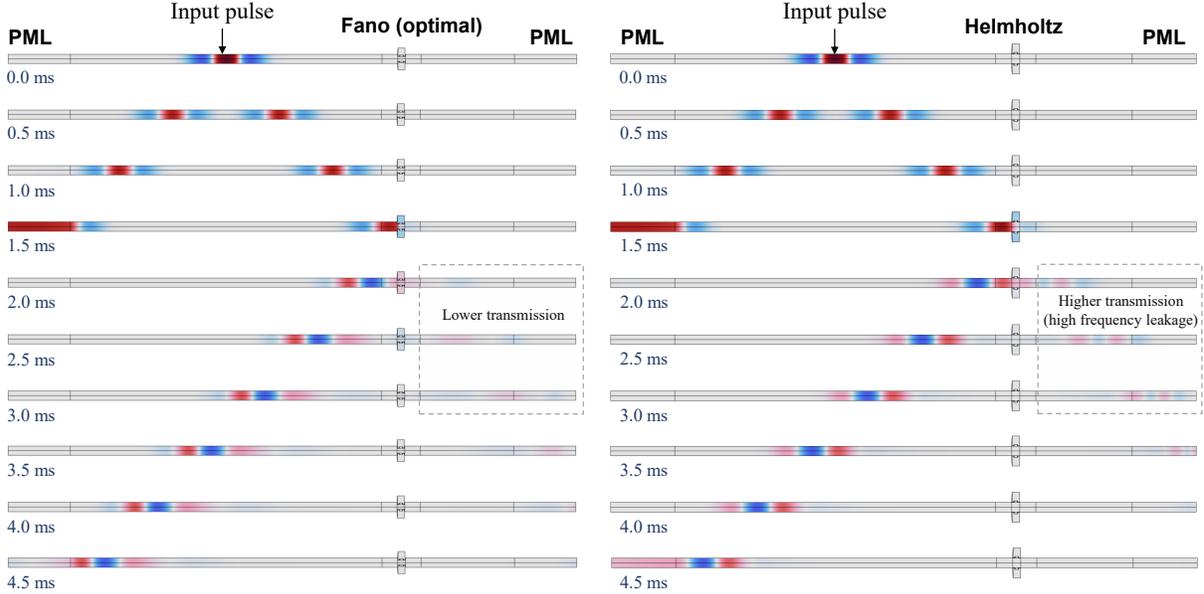

FIG. S6: The time-domain FEM simulation results from 0 ms to 4.5 ms. Ricker's Wavelet as initial incident waves  $p_{\text{in}}(x) = \left(1 - \frac{x^2}{B^2}\right) e^{-\frac{x^2}{2B^2}}$ , where  $B^2 = \frac{c_0^2}{2\pi^2 f_0}$  (Broadband Pulse centered at  $f_0$ ). PML: perfect matching layer.

#### S3-4. Time-domain simulation (Helmholtz and Fano types)

Time-domain simulations were conducted using the 'Pressure Acoustics, Time Explicit' interface to capture the transient response of the system. The numerical study spanned a duration from 0 ms to 4.5 ms. To analyze the broadband response, a Ricker wavelet was utilized as the incident source, governed by the equation  $p_{\text{in}}(x) = \left(1 - \frac{x^2}{B^2}\right) e^{-\frac{x^2}{2B^2}}$ , with the width parameter defined as  $B^2 = \frac{c_0^2}{2\pi^2 f_0}$ . This pulse is centered at a frequency of  $f_0 = 3600$  Hz. To simulate an open domain, Perfectly Matched Layers (PMLs) were implemented at the two terminations of the main duct.

Figure (S6) visualizes the temporal evolution of the acoustic field for both Helmholtz and Fano-type resonators, maintaining the geometric dimensions used in the frequency domain analysis. While both structures demonstrate sound blocking and scattering capabilities, their mechanisms differ significantly. The Helmholtz resonator exhibits a narrow stopband with a peak transmission loss (TL) near 1600 Hz. In contrast, the Fano resonator produces a broadband back-scattering spectrum [see Fig. S7(a-c)]. The time-domain visualization confirms that the optimally tuned Fano resonator results in significantly lower transmission leakage compared to the Helmholtz design. Notably, the snapshot of the Helmholtz resonator reveals significant transmission of high-frequency components downstream; this is visually identifiable by the reduced spatial distance between wave nodes, corresponding to shorter wavelengths passing through the system.

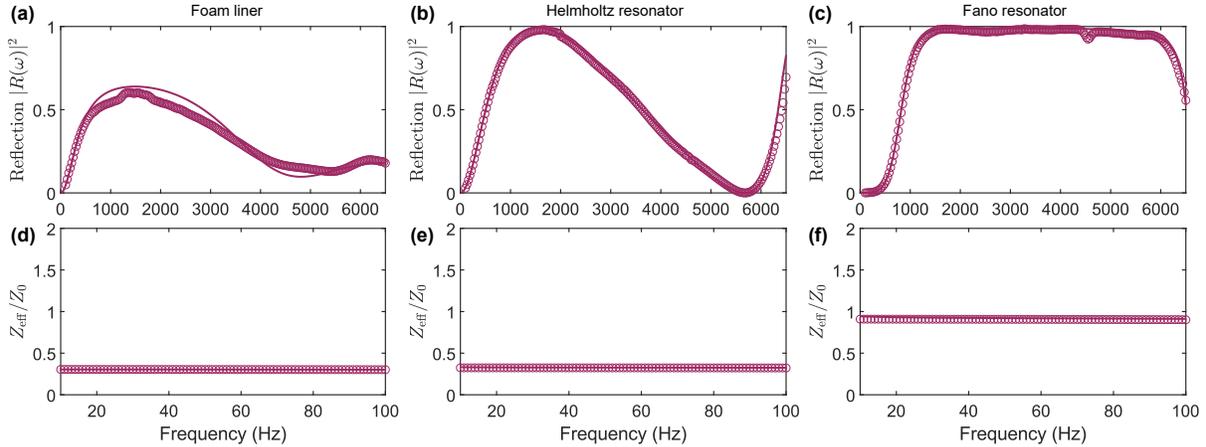

FIG. S7: Reflection coefficient, complementary to the transmission coefficient, and impedance matching mechanism for Fano-resonance-based spectral shaping. (a–c)  $|R(\omega)|^2$  for the foam liner, Helmholtz resonator, and optimal Fano resonator. (d–f) The corresponding data for  $Z_{\text{eff}}(\omega) (= \sqrt{\rho_{\text{eff}}(\omega)M_{\text{eff}}(\omega)})$  in the quasi-static band below 100 Hz, obtained using the extraction method presented in Table (S1). Only (c) and (f) satisfy the optimal Fano interference condition, which approximately matches the impedance of air at the static limit. The circles are from experiments while the solid lines are extracted from FEM simulation.

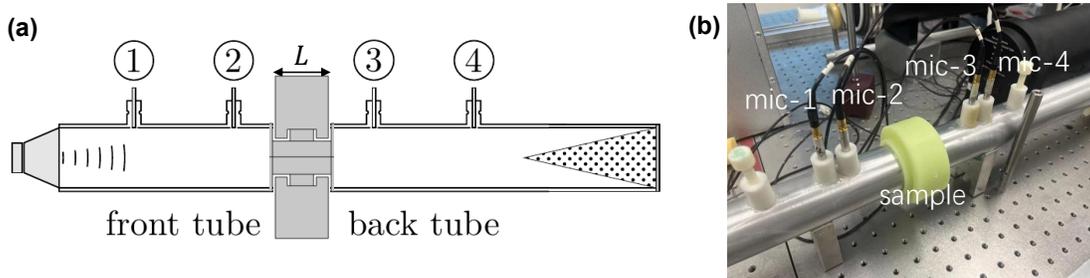

FIG. S8: The experimental setups based on the four-microphone method. (a) Schematic of the impedance tube (circular, 3 cm diameter). (b) Photograph of the testing device. The end of the impedance tube is filled with a porous foam wedge, with a length of 1 m, to mimic a perfectly matched layer (sufficient to absorb sound waves from 100 Hz and above).

## S4. Impedance tube measurements

### S4-1. Sample fabrication

The fabrication of the sample frame [see Fig. (S5b)] was facilitated by employing 3D printing technology, specifically Stereolithography (SLA) using WeNext 8228 Resin. This method provided the precision required to accurately resolve features such as narrow channels and necks with dimensions smaller than 0.4 mm. The resulting structures exhibited sufficient rigidity to be considered as hard boundaries in the context of acoustic fields.

### S4-2. Experimental setup: standard four microphone method

In this experiment [see Fig. (S8)], a custom-built impedance tube featuring a circular cross-section with a diameter of 3 cm was utilized. The experimental setup included BSWA microphones (model MPA416), NI sound cards (model CompactDAQ9263), and an NI acquisition card (model CompactDAQ9234). Harmonic sine waves were produced using a HIVI speaker (model M3N) in combination with a YAMAHA power amplifier (model PX3). The acoustic properties of the samples were assessed through a standard four-microphone technique within the impedance tube measurements. Prior to each series of experiments, microphone mismatch calibration was conducted meticulously in accordance with established standards (ASTM E2611-09). To mitigate noise interference caused by leakage, Plasticine was applied to seal all potential connection gaps. Moreover, the cut-off frequency of the impedance tube was determined to be 6700 Hz, slightly exceeding the upper frequency limit of our absorption measurements (6500 Hz). Data below 100 Hz were excluded due to the challenges and inaccuracies associated with low-frequency measurements.

### S4-3. Data post-processing: sum-rule-based Padé model fitting

To fit the experimental data  $(\omega_j, y_j)$  ( $K$  points) where  $y_j = 2(1 - T(\omega_j))$  using a sum-rule-constrained Padé model, we introduce a scaling factor  $\Gamma$  to nondimensionalize the frequency, defining

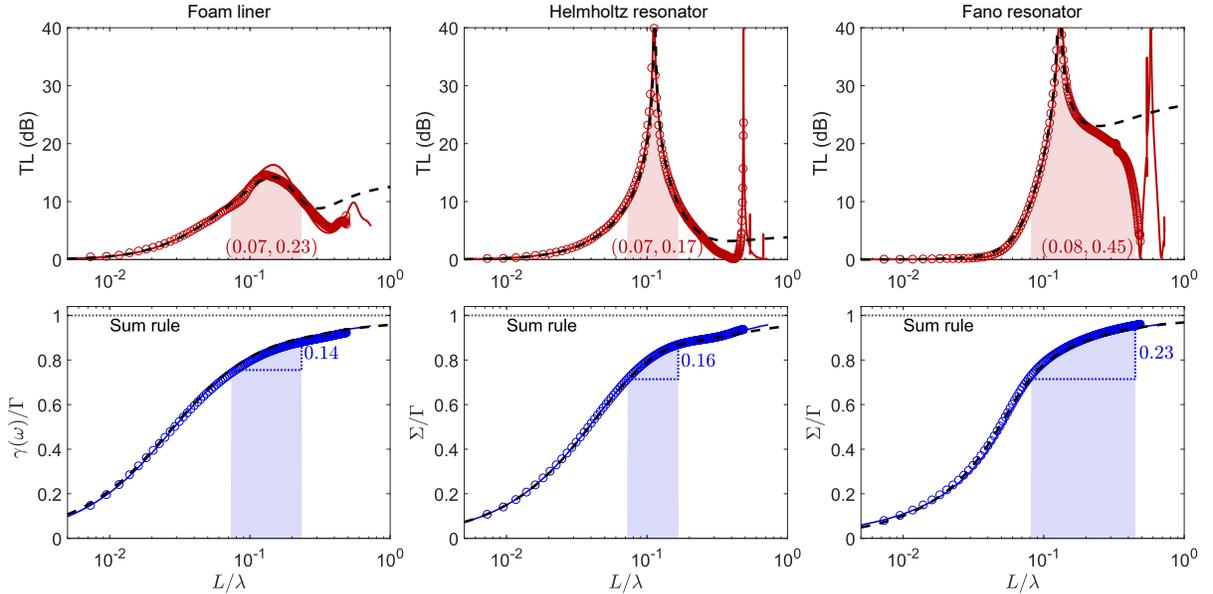

FIG. S9: The transmission loss data (first row) and the cumulative distribution function  $\gamma(\omega)$  (second row). The three columns correspond to the foam liner, the Helmholtz resonator, and the optimal Fano resonator, respectively. The adopted formula (data presented by circles) was that  $\gamma(\omega) = \int_{2\pi \times 100}^{\omega} \sigma_{\text{exp}}(\omega) \frac{d\omega}{\omega^2} + \Delta\gamma_{\text{simu}}$ , where  $\sigma_{\text{simu}}, \sigma_{\text{exp}}$  denote absorption spectra from simulation and experiments respectively and  $\Delta\gamma_{\text{simu}} = \int_0^{2\pi \times 100} \sigma_{\text{simu}}(\omega) \frac{d\omega}{\omega^2}$ . The dashed lines denote fitting model from the Table. (S3).

the complex variable as  $s \equiv -i\tilde{\omega} = -i\omega\Gamma$ . The transfer function is expressed as:

$$H(s) = \frac{\sum_{k=1}^m \tilde{a}_k s^k}{1 + \sum_{k=1}^n \tilde{b}_k s^k}. \quad (\text{S28})$$

In this formulation, the first numerator coefficient is fixed by the sum rule as

$$\tilde{a}_1 = \frac{2}{\pi}. \quad (\text{S29})$$

Consequently, this term is treated as a known constant rather than a fitting parameter. The error equation  $N(s_j) - y_j D(s_j) \approx 0$  is linearized and rearranged to isolate the unknown coefficients on the left-hand side:

$$\sum_{k=2}^m \tilde{a}_k s_j^k - \sum_{k=1}^n \tilde{b}_k (y_j s_j^k) \approx y_j - \tilde{a}_1 s_j. \quad (\text{S30})$$

This leads to a modified overdetermined linear system  $\mathbf{A}\mathbf{x} = \mathbf{b}$ . The unknown coefficient vector is reduced to  $\mathbf{x} = [\tilde{a}_2, \dots, \tilde{a}_m, \tilde{b}_1, \dots, \tilde{b}_n]^T$ . The observation vector  $\mathbf{b}$  is adjusted to account for the fixed  $\tilde{a}_1$  term:

$$\mathbf{b} = \begin{bmatrix} y_1 - \tilde{a}_1 s_1 \\ \vdots \\ y_K - \tilde{a}_1 s_K \end{bmatrix}. \quad (\text{S31})$$

The system matrix  $\mathbf{A}$  is constructed starting from the second power of  $s$  for the numerator part:

$$\mathbf{A} = \begin{bmatrix} s_1^2 & \dots & s_1^m & -y_1 s_1 & \dots & -y_1 s_1^n \\ \vdots & \ddots & \vdots & \vdots & \ddots & \vdots \\ s_K^2 & \dots & s_K^m & -y_K s_K & \dots & -y_K s_K^n \end{bmatrix}. \quad (\text{S32})$$

To estimate the optimal coefficients vector  $\mathbf{x}$  for the overdetermined system derived from frequency response measurements, we employ the Least Squares method to minimize the residual error vector defined as  $\mathbf{e} = \mathbf{b} - \mathbf{A}\mathbf{x}$ . The objective is to minimize the cost function  $J(\mathbf{x}) = |\mathbf{e}|^2 = (\mathbf{b} - \mathbf{A}\mathbf{x})^H (\mathbf{b} - \mathbf{A}\mathbf{x})$ , where  $(\cdot)^H$  denotes the Hermitian transpose. By expanding this quadratic form to  $J(\mathbf{x}) = \mathbf{b}^H \mathbf{b} - \mathbf{b}^H \mathbf{A}\mathbf{x} - \mathbf{x}^H \mathbf{A}^H \mathbf{b} + \mathbf{x}^H \mathbf{A}^H \mathbf{A}\mathbf{x}$  and setting the gradient with respect to  $\mathbf{x}$  to zero, specifically  $\nabla_{\mathbf{x}} J(\mathbf{x}) = -2\mathbf{A}^H \mathbf{b} + 2(\mathbf{A}^H \mathbf{A})\mathbf{x} = 0$ , we derive the Normal Equation  $(\mathbf{A}^H \mathbf{A})\mathbf{x} = \mathbf{A}^H \mathbf{b}$ . Assuming the system matrix  $\mathbf{A}$  has full column rank, the matrix  $\mathbf{A}^H \mathbf{A}$  is invertible, yielding the

TABLE S3: The fitted  $3 \times 3$  Padé coefficients of  $2(1 - T(\tilde{\omega}))$  for different acoustic devices by using Eq. (S33).

| Devices   | Numerator coefficients |               |               |               | Denominator coefficients |               |               |               |
|-----------|------------------------|---------------|---------------|---------------|--------------------------|---------------|---------------|---------------|
|           | $\tilde{a}_0$          | $\tilde{a}_1$ | $\tilde{a}_2$ | $\tilde{a}_3$ | $\tilde{b}_0$            | $\tilde{b}_1$ | $\tilde{b}_2$ | $\tilde{b}_3$ |
| Foam      | 0                      | $2/\pi$       | 0.05060       | 0.00790       | 0.31831                  | 0.34260       | 0.03119       | 0.00325       |
| Helmholtz | 0                      | $2/\pi$       | 0.04861       | 0.01541       | 0.31831                  | 0.28400       | 0.05075       | 0.00474       |
| Fano      | 0                      | $2/\pi$       | 0.24687       | 0.06413       | 0.31831                  | 0.29656       | 0.14419       | 0.03073       |

closed-form optimal solution:

$$\mathbf{x} = (\mathbf{A}^H \mathbf{A})^{-1} \mathbf{A}^H \mathbf{b}. \quad (\text{S33})$$

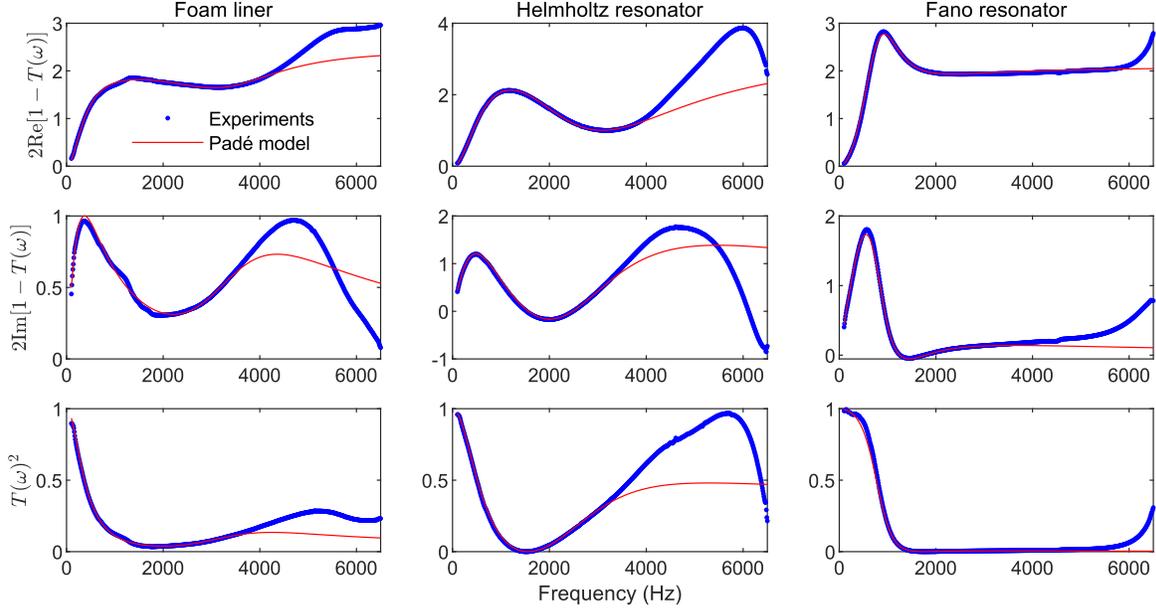

FIG. S10: The decomposition of the real and imaginary parts of the transmission-based data (blue points). (a) The measured  $2 \operatorname{Re}[1 - T(\omega)]$  (i.e.,  $\sigma_{\text{ext}}(\omega)$ ) and its Padé model fit (red line). (b) The measured  $2 \operatorname{Im}[1 - T(\omega)]$  and its Padé model fit (red line). The fitting range is from 100 Hz to 4000 Hz, using a minimal Padé order of  $[3 \times 3]$ , as per Table (S2).

#### S4-4. Additional analysis of the measured data

Theoretically, if we have an infinite number of orders, we can fit the transmission transfer function that conforms to human causality. However, real-world data always requires some truncation. Here, we chose  $m = 3$ ,  $n = 3$  as the simplest fitting order, as we have justified in End Matter of the main text, while not losing the physical picture of Fano resonance (coupling and interference between the two modes). In Table (S3), for the three cases (foam, Helmholtz and Fano resonator), the fitting formula is

$$2(1 - T(\tilde{\omega})) = \frac{\tilde{a}_1(i\tilde{\omega}) + \tilde{a}_2(i\tilde{\omega})^2 + \tilde{a}_3(i\tilde{\omega})^3}{1 + \tilde{b}_1(i\tilde{\omega}) + \tilde{b}_2(i\tilde{\omega})^2 + \tilde{b}_3(i\tilde{\omega})^3}, \quad (\text{S34})$$

where  $\tilde{\omega} = \omega\Gamma$ . Also, we observed the reported Fano resonance-based transmission [7] also followed this relation:  $T(\omega) = \left[1 - i\omega \left(\sqrt{b} + \frac{\alpha}{\omega_m^2 - \omega^2 - i\beta\omega}\right)\right]^{-1}$  ( $\beta = 0$  for lossless scatterer), which is equivalent to the form of Eq. (6) in Ref. [7]:

$$|T(\omega)|^2 = \frac{(\omega^2 - \omega_m^2)^2}{(\omega^2 - \omega_m^2)^2 + \omega^2 \left[\sqrt{b}(\omega^2 - \omega_m^2) - \alpha\right]^2}. \quad (\text{S35})$$

Based on our experiments, the fitting results are shown in Fig. (S10) and Table (S3). It can be seen that the fitted curve matches the experimental results well at low frequencies (100-4000Hz). At higher frequencies, a higher order would likely result in an even better fit. However, we have already obtained very good fitting parameters for the Fano resonance curve. The third column of Fig. (S10) shows an excellent fit. Furthermore, our fitting process ensures that the sum rule always holds. Therefore, the degrees of freedom generated by the Fano resonance are well captured. Additionally, in Fig. (S9), we have also labeled the transmission loss corresponding to the fitting model on the logarithmic frequency axis. As we understand conventional resonance (e.g., Helmholtz) and Fano resonance, the former has a nearly symmetrical line shape, while the latter has an asymmetrical curve.

- 
- [1] A. Baldin, Polarizability of nucleons, *Nuclear Physics* **18**, 310 (1960).
  - [2] B. R. Holstein and S. Scherer, Hadron polarizabilities, *Annual Review of Nuclear and Particle Science* **64**, 51 (2014).
  - [3] J.-P. Groby, M. Mallejac, A. Merkel, V. Romero-García, V. Tournat, D. Torrent, and J. Li, Analytical modeling of one-dimensional resonant asymmetric and reciprocal acoustic structures as willis materials, *New Journal of Physics* **23**, 053020 (2021).
  - [4] M. Yang, G. Ma, Y. Wu, Z. Yang, and P. Sheng, Homogenization scheme for acoustic metamaterials, *Physical Review B* **89**, 064309 (2014).
  - [5] S. Qu, M. Yang, T. Wu, Y. Xu, N. Fang, and S. Chen, Analytical modeling of acoustic exponential materials and physical mechanism of broadband anti-reflection, *Materials Today Physics* **44**, 101421 (2024).
  - [6] B. Friedland, *Control system design: an introduction to state-space methods* (Courier Corporation, 2012).
  - [7] C. Goffaux, J. Sánchez-Dehesa, A. L. Yeyati, P. Lambin, A. Khelif, J. Vasseur, and B. Djafari-Rouhani, Evidence of fano-like interference phenomena in locally resonant materials, *Physical review letters* **88**, 225502 (2002).
  - [8] G. W. Milton, *The Theory of Composites* (Society for Industrial and Applied Mathematics (SIAM), 2022).
  - [9] X. Zhou and G. Hu, Analytic model of elastic metamaterials with local resonances, *Physical Review B—Condensed Matter and Materials Physics* **79**, 195109 (2009).
  - [10] P. Sheng, J. Mei, Z. Liu, and W. Wen, Dynamic mass density and acoustic metamaterials, *Physica B: Condensed Matter* **394**, 256 (2007).
  - [11] S. Qu, M. Yang, S. Huang, S. Liu, E. Dong, H. Y. Li, P. Sheng, I. D. Abrahams, and N. X. Fang, Generalized causality constraint based on duality symmetry reveals untapped potential of sound absorption, *Nature Communications* **16**, 10749 (2025).
  - [12] C. Ge, N. Wang, X. Wang, and Y. Li, Causal-constraint broadband sound absorption under isothermal process, *Physical Review Letters* **134**, 237001 (2025).
  - [13] N. Fang, D. Xi, J. Xu, M. Ambati, W. Srituravanich, C. Sun, and X. Zhang, Ultrasonic metamaterials with negative modulus, *Nature materials* **5**, 452 (2006).
  - [14] Z. Liu, X. Zhang, Y. Mao, Y. Y. Zhu, Z. Yang, C. T. Chan, and P. Sheng, Locally resonant sonic materials, *science* **289**, 1734 (2000).
